# Supplementary material for: Mitigating over-exploration in latent space optimization using LES
Source: arXiv:2406.09657 source file (2025-02-21)
Supplement: Supplementary file 1 [file ds.tex]

\input{arxiv/tables/lso_bm}
