# Supplementary material for: Mitigating over-exploration in latent space optimization using LES
Source: arXiv:2406.09657 source file (2025-02-21)
Supplement: Supplementary file 2 [file wall_clock.tex]

\paragraph{Resources and wall clock times} All the experiments in this works were carried out using a single GPU (NVIDIA A100).
